# Supplementary material for: ELMGS: Enhancing memory and computation scaLability through coMpression for 3D Gaussian Splatting
Source: arXiv:2410.23213 source file (2024-10-30)
Supplement: Supplementary file 1 [file memory_consumption.tex]

\begin{figure*}[t]
    \centering
    \includegraphics[width=0.5\linewidth]{figures/Supplementary_Figures/Memory_Consumption.pdf}
    \caption{Memory savings while training using Gradient and Opacity based Pruning (GAP) on Tanks\&Temples dataset.}
    \label{sup-fig:memory_savings}
    \vspace{-10pt}
\end{figure*}
